# Supplementary material for: Concentration Network for Reinforcement Learning of Large-Scale Multi-Agent Systems
Source: arXiv:2203.06416 source file (2022-04-07)
Supplement: Supplementary file 1 [file ____________.pdf]

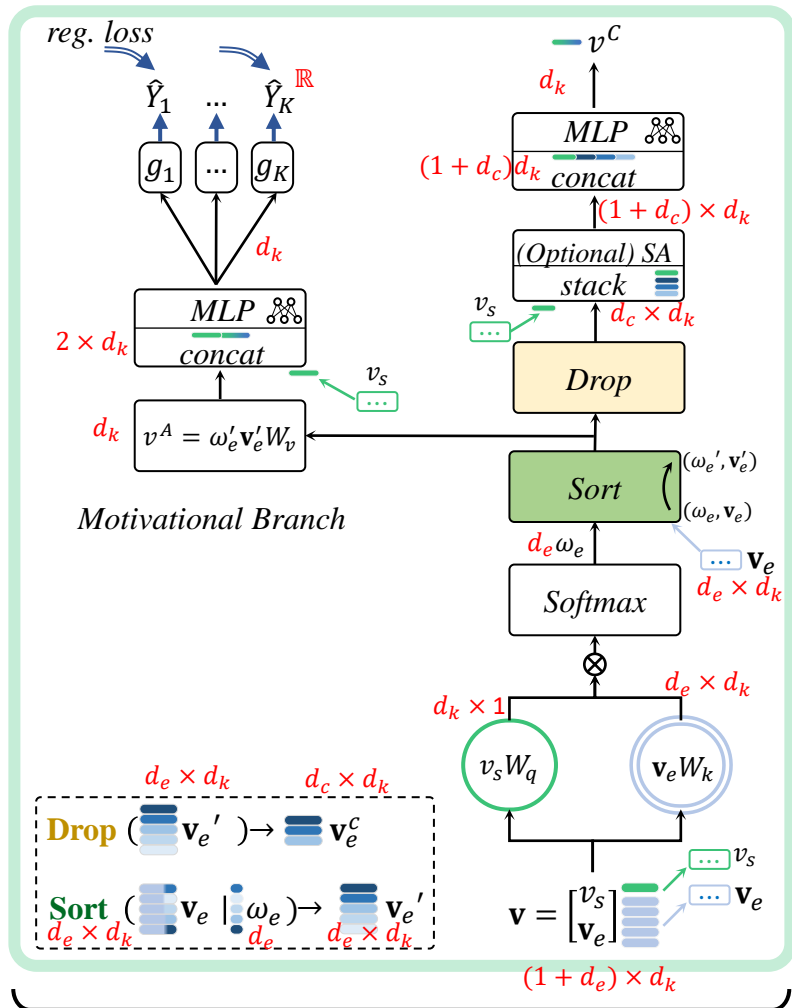

Concentration Module

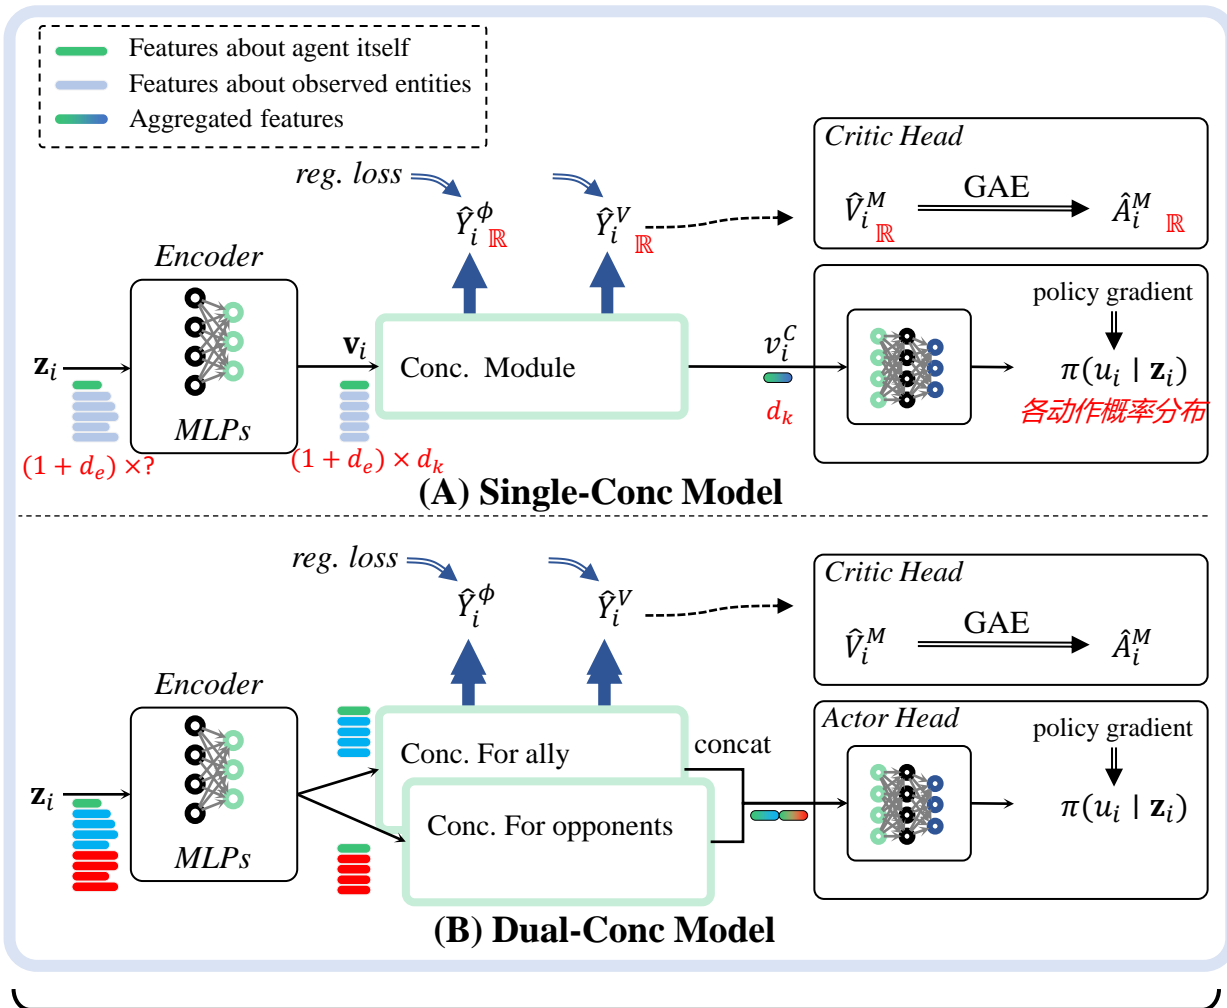

Concentration-Based Policy Gradient Models

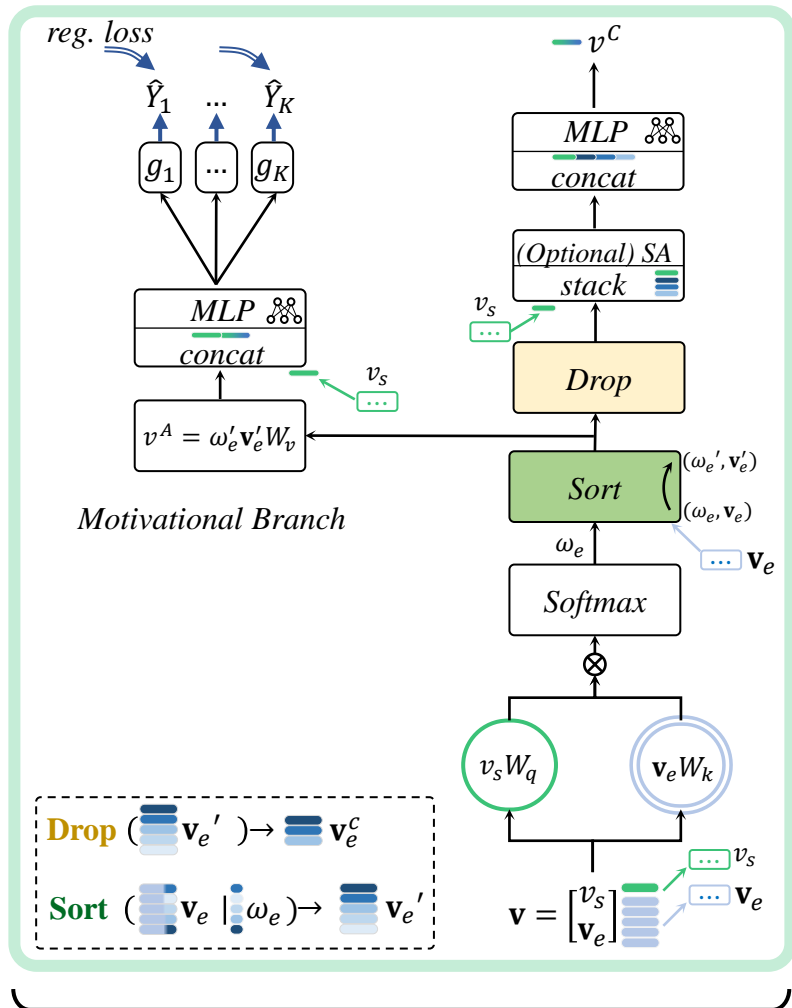

Concentration Module

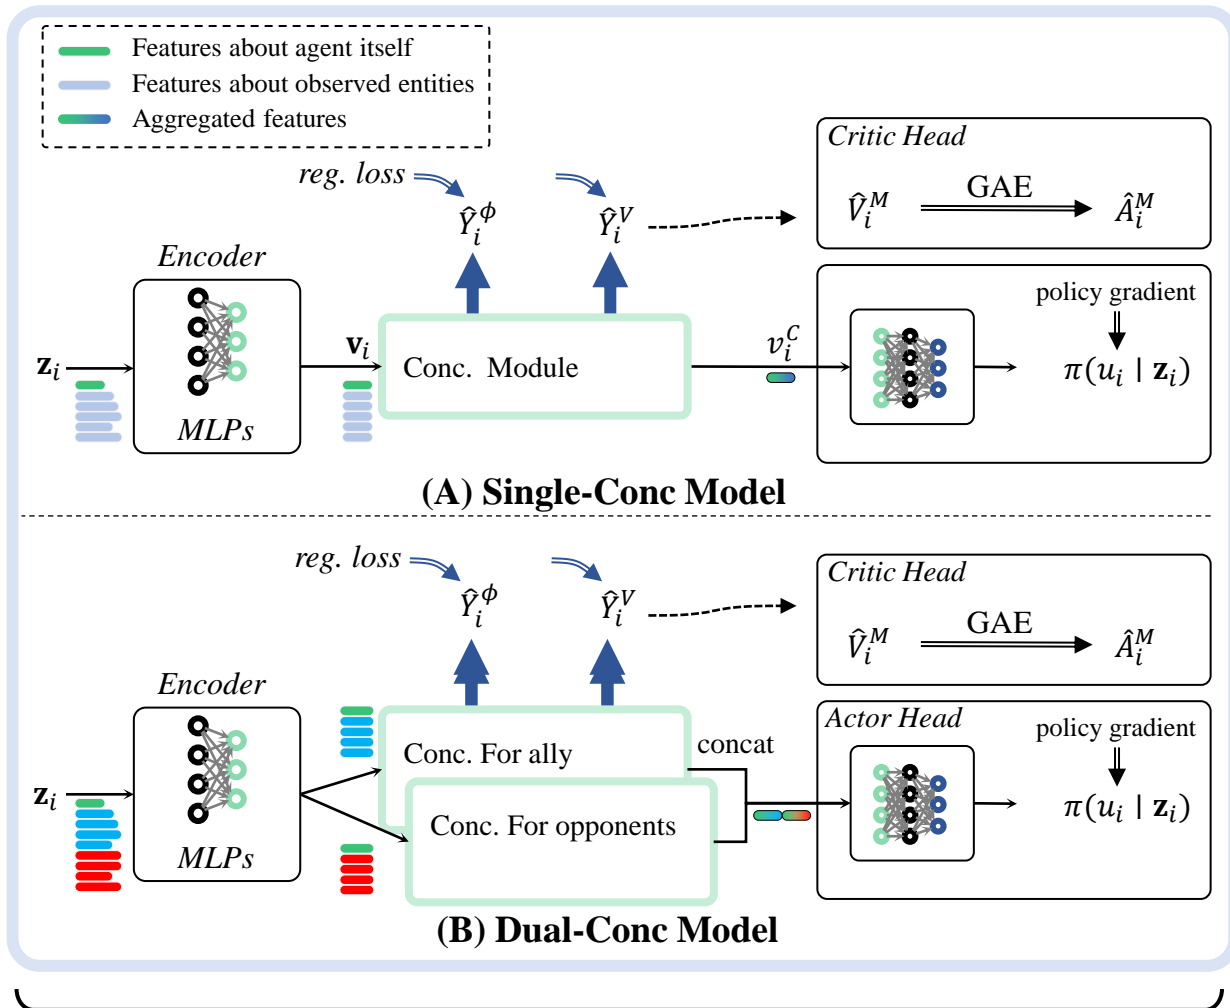

Concentration-Based Policy Gradient Models
